# Supplementary material for: Cone-Copositive Lyapunov Functions for Complementarity Systems: Converse Result and Polynomial Approximation
Source: arXiv:2104.06360 source file (2021-04-13)
Supplement: Supplementary file 1 [file appendixB.tex]

% !TEX root = sosCertEVIs.tex
%%%%%%%%%%%%%%%%%%%%%%%%%%%%%%%%%%%
\appendix

\begin{proof}[Proof of Lemma~\ref{lem:contproperty}]
First, since $W$ is continuous over a compact set and $f$ is locally bounded then $M$ is well defined. And since $W$ is a Lyapunov function then $M > 0$.

Using the homogeneity of $W$, it gives $ \nabla W (y). y = d. W(y)$ and by the reason of $W(y)=1$, we obtain
\[
\nabla W (y). y = d
\]
which implies
\[
\nabla W (y). x = d-\nabla W (y). (y-x),
\]
and then the assumption $\nabla W(y) . x > d- \delta$ is equivalent to $\nabla W (y). (y-x) < \delta$.

Interpreting by contradiction, suppose that there exists a sequence $(x_i,y_i,f_j)$ such that $\nabla W(y_i).f_i(x_i) \ge -\epsilon$ and $\nabla W (y_i). (y_i-x_i) \rightarrow 0$ as $j \rightarrow \infty $.
By Bolzano-Weierstrass theorem in real analysis, we can find a subsequence of $(x_i,y_i,f_j)$ that converges to $(\bar{x},\bar{y},\bar{f})$. As a consequence, by continuity we get $\nabla W(\bar{y}). \bar{f}(\bar{x}) \ge -\epsilon$ and $\nabla W (\bar{y}). (\bar{y}-\bar{x}) = 0$.

The equation $\nabla W (\bar{y}). (\bar{y}-\bar{x}) = 0$ means that $\bar{y}-\bar{x}$ belongs to the tangent space at $\bar{y}$ of the strictly convex set $W^{-1}([0,1])$. Moreover we have that $\bar{x}$ is also on the boundary of this set then it should be $\bar{y}=\bar{x}$. From this, we get a contradiction seeing that  $\nabla W(\bar{y}). \bar{f}(\bar{x})= \nabla W(\bar{x}). \bar{f}(\bar{x}) \le -M$.

\end{proof}
We take $\delta \in (0,1)$ compatible to some $\epsilon$ in the lemma~\ref{lem:contproperty}, and for every $y \in W^{-1}(1)$, let $B_y = \left\{x \in \R^n \vert\ \nabla W (y) . x > 1-\frac{\delta}{2} \right\}$ the open sets. We have $y \in B_y$ so $\left\{ B_y \right\}_{y \in W^{-1}(1)}$ is an open covering of $W^{-1}(1)$. And then we can find $y_1,...,y_N$ points of $W^{-1}(1)$ such that the union of $B_{y_k}$, $k=1,...,N$, covers $W^{-1}(1)$.

Let us define
\[
\wt W(x) = \sum_{k=1}^{N} (\nabla W (y_k).x)^{2p}.
\]
For a large integer $p$, we affirm that $\wt W$ is a polynomial Lyapunov function.

For $f \in \textrm{LB}(\R^n)$ and $x \in \R^n$ such that $x \ne 0$, we have
\[
\wt W(x) . f(x) = 2p \sum_{k=1}^{N} (\nabla W (y_k).x)^{2p-1} \nabla W (y_k) . f(x).
\]
We need to prove that $\left\langle \nabla \wt W (x), f(x) \right\rangle < 0$. Since we have homogeneity, we can prove it just for $x \in W^{-1}(1)$. Let us introduce
\[
K := \max_{ x,y \in W^{-1}(1) f \in \textrm{LB}(\R^n)} [-\nabla W(y).f(x)].
\]
If for some $k \in \left\{1,...,N\right\}$, we have $\vert \nabla W(y_k) . x \vert \le d - \delta$, then
\[
\vert(\nabla W (y_k).x)^{2p-1} \nabla W (y_k) . f(x) \vert \le (d-\delta)^{2p-1} K.
\]
In other way, if $d- \frac{\delta}{2} \ge \vert \nabla W (y_k) . x \vert > d- \delta$, then, we can use lemma~\ref{lem:contproperty}. Therefore the term in the summation is negative.

Since there exist at least two distinct indices $k_1$ and $k_2$ such that $x \in B_{y_{k_1}}$ and $-x \in B_{y_{k_2}}$, we have
\[
(\nabla W (y_{k_i}).x)^{2p-1} \nabla W (y_{k_i}) . f(x) < -(d- \frac{\delta}{2})^{2p-1} \epsilon.
\]
Finally, we obtain that
\begin{align*}
\nabla & \wt W (x) . Dx  < 2p \left(-2(d-\delta/ 2)^{2p-1} \epsilon + (N-2)(d-\delta)^{2p-1} K \right) \\
& = -4p(d-\delta / 2)^{2p-1} \epsilon \left( 1- \frac{K(N-2)}{2 \epsilon} \left (\frac{d-\delta}{d-\delta /2} \right)^{2p-1} \right).
\end{align*}
For $p$ large enough, the right-hand side of the previous inequality is negative. Then the theorem~\ref{thm:converseMain} is proved.

\end{proof}
